# Supplementary material for: Evaluating Stability in Massive Social Networks: Efficient Streaming Algorithms for Structural Balance
Source: arXiv:2306.00668 source file (2023-06-01)
Supplement: Supplementary file 1 [file appendix-alt-proof-S-sampler.tex]

\section{A Combinatorial Proof of \Cref{lem:neg-sample}}
\label{app:alt-proof}
Suppose $G$ is balanced, then either the graph $\Gm$ is empty, or it is a complete bipartite graph. In the first case, the number of $\mlab$ edges in $G[S]$ is always $0$. In the second case, let $L$ and $R$ be the bi-partition of $\Gm$, and let $A=L\cap S$ and $B=R\cap S$. Observe that one of $A$ and $B$ must have odd number of vertices while the other have even (since $\card{S}$ is odd). Assume w.log. that $\card{A}$ is even and $\card{B}$ is odd, since $\Gm[S]$ is an induced subgraph of a complete bipartite graph, $\Gm[S]$ itself must also be complete bipartite. As such, the number of negative edges must be $\card{A}\cdot \card{B}$, which is an even number.

% we would like to show $\card{\Em_G\paren{S}} \equiv 0 \mod 2$. There are two possibilities for a balanced graph: all edges have \plab sign or there exists a partition of sampled vertices $S = (A, B)$ such that every edge $(u,v)$ is labeled \mlab where $u\in A, v\in B$, and the rest is labeled \plab. For the first case $\card{\Em_G\paren{S}} = 0$; For the second case, one of the partitions must have odd number of vertices while the other have even, since $\card{S}$ is odd. Let us assume $\card{A}$ is even and $\card{B}$ is odd. Note the induced subgraph of $G$ on $S$ is also a complete graph, therefore the amount of negative edges is $\card{A}\cdot \card{B}$, which is an even number.

We now prove the correctness for the case when $G$ is not balanced. Let $\Em(S')$ denote the set of \mlab edges sampled by the $S$-sampler inside $S'$, and let $\Em(v_n, S')$ be the set of \mlab edges between $v_n$ and $S'$. (Recall $v_{n}$ is the special vertex we choose such that its inclusion of $S$ is dependent on the parity of $S'$.) Our strategy is to show to analyze the cases for the parity of $\card{\Em(S')}$ and $\card{\Em(v_n, S')}$, and show that with at least $\frac{1}{4}$ probability the parity of \mlab edges is odd in all cases. % Our strategy is to show that with at least $\frac{1}{4}$ probability, the parity of $\card{\Em(S')}$ and $\card{\Em(v_n, S')}$ are different (i.e. odd and even). As such, the final parity of the number of \mlab edges is odd with probability at least $\frac{1}{4}$.

Let $N^{+}_{G}(v_n)$ be the set of vertices (in $G$ and independent of the $S$-sampler) that connect to $v_n$ with \plab edges, and let $N^{-}_{G}(v_n)$ be the set of vertices with \mlab edges. Since $G$ is not balanced, the induced subgraph of $G[N^{+}_{G}(v_n) \cup N^{-}_{G}(v_n)]$ \vik{Is this just $G$ induced on every vertex besides $v_n$? If yes, this claim is false; it can be complete bipartite (I am assuming you meant either the graph using \mlab edges is complete bipartite).} is \emph{not} complete bipartite \vik{Ok, I think I know what you're trying to say. It's not the case that there are all \mlab edges between $N^+$ and $N^-$ and no \mlab edges inside. The notation used is wrong however}.
As such, we must be in either \underline{scenario $(A).$} an edge $(u,v)\in \Em$ such that either both $(u,v) \in N^{+}_{G}(v_n)$ or $(u,v) \in N^{-}_{G}(v_n)$ or \underline{scenario $(B).$} there exists a vertex pair $(u,v)$ such that $u \in N^{+}_{G}(v_n)$ and $v \in N^{-}_{G}(v_n)$, and $(u,v)\not\in \Em$. We discuss the cases respectively. 

\subsubsection*{The cases in \underline{scenario $(A).$}}
Fix all the coins in $S'$ used by line~\ref{line:S-sample-indep} of the $S$-sampler \emph{except} for the special $u$ and $v$ in scenario $(A)$, and observe that we sample $u$ and $v$ independently with probability $\frac{1}{2}$ each. We analyze the two cases separately. 

\paragraph{The case of $(u,v) \in N^{+}_{G}(v_n)$.} In this case, the sampling of $u$ and $v$ is independent of the parity of $\card{\Em(v_n, S')}$. Therefore, we only need to show that the number of \mlab edges in $\Em(S')$ is odd or even with probability at least $\frac{1}{4}$ each. We prove the case for the odd number since the even number follows the same argument. If the number of \mlab edges sampled by $S' \setminus \{u,v\}$ is odd, then with probability at least $\frac{1}{4}$, we do not sample neither of $u$ and $v$. As such, the number of \mlab edges remains odd \vik{Wouldn't we need to consider the role of $v_n$? After the coins for $u$ and $v$ are flipped, $v_n$ might be included and flip the parity.}. On the other hand, if the number of \mlab edges sampled by $S' \setminus \{u,v\}$ is even, we have
\begin{enumerate}[label=\Alph*).,leftmargin=1.5cm]
\item If one of $(u,v)$ has an odd number of \mlab edges connecting to $S'\setminus \{u,v\}$ (and suppose w.log. that this vertex is $v$), then with probability at least $\frac{1}{4}$, we sample $v$ but not $u$, which gives us an odd number of \mlab edges.
\item If both of $(u,v)$ has an even number of \mlab edges connecting to $S'\setminus \{u,v\}$, then with probability at least $\frac{1}{4}$, we sample both $u$ and $v$, which gives us an odd number of \mlab edges since there is one extra \mlab edge between $u$ and $v$.
\end{enumerate}
\vik{The above should explicate the role of $v_n$. Sampling $u$ and $v$ are independent of the parity of $\card{\Em(v_n, S')}$. But they are not independent of the pairty of $\card{\Em(V_n, S')}$ where including $v_n$ or not determines whether an event happens.}

\paragraph{The case of $(u,v) \in N^{-}_{G}(v_n)$.}  In this case, the sampling of $u$ and $v$ will affect the parity of $\card{\Em(v_n, S')}$. Therefore, we need a more detailed case discussion as follows.
\begin{enumerate}[label=\Alph*).,leftmargin=1.5cm]
\item The cases when the number of vertices in $S'\setminus \{u,v\}$ is odd:
\begin{enumerate}
\item Suppose there is an even number of vertices sampled from $N^{-}_{G}(v_n)$ in $S'\setminus \{u,v\}$. In this case, if the number of \mlab edges sampled by $S' \setminus \{u,v\}$ is odd, then with probability $\frac{1}{4}$, we do not sample neither of $\{u,v\}$ and we do not sample $v_n$. As such, the total number of \mlab edges is odd. Otherwise, if the number of \mlab edges sampled by $S' \setminus \{u,v\}$ is even, and $(u,v)$ have different parities of \mlab edges connecting to $S' \setminus \{u,v\}$ (suppose w.log. $v$ has an odd number of \mlab edges); then, with probability at least $\frac{1}{4}$ we sample $v$ but not $u$, and $v_n$ will be sampled. As such, the total parity of the \mlab edges is odd \vik{Shouldn't it be $u$ and not $v$? Adding $u$ increases \mlab edges by an even number (i.e. does not change parity). Now there are an odd number of things in $N^-$. Including $v_n$ consequently flips the parity.}. Finally, if the number of \mlab edges sampled by $S' \setminus \{u,v\}$ is even and $(u,v)$ have the same parity of \mlab edges connecting to $S' \setminus \{u,v\}$, then with probability at least $\frac{1}{4}$ both $u$ and $v$ are sampled and $v_n$ is not sampled. As such, the total parity of the \mlab edges is again odd as $(u,v)\in E^-$.
\item Suppose there is an odd number of vertices sampled from $N^{-}_{G}(v_n)$ in $S'\setminus \{u,v\}$. The analysis is the same with case $(a)$ except when the number of \mlab edges sampled by $S' \setminus \{u,v\}$ is even and $(u,v)$ have different parities of \mlab edges connecting to $S' \setminus \{u,v\}$, we count the case of sampling the vertex with an odd number of edges connecting to $S' \setminus \{u,v\}$, which happens with probability at least $\frac{1}{4}$.
\end{enumerate}
\item The cases when the number of vertices in $S'\setminus \{u,v\}$ is even:
\begin{enumerate}
\item If there is an even number of vertices sampled from $N^{-}_{G}(v_n)$ in $S'\setminus \{u,v\}$. In this case, if the number of \mlab edges sampled by $S' \setminus \{u,v\}$ is odd, then with probability $\frac{1}{4}$, we do not sample neither of $\{u,v\}$ and we sample $v_n$. As such, the total number of \mlab edges is odd. Otherwise, if the number of \mlab edges sampled by $S' \setminus \{u,v\}$ is even, and $(u,v)$ have different parities of \mlab edges connecting to $S' \setminus \{u,v\}$ (suppose w.log. $v$ has an odd number of \mlab edges); then, with probability at least $\frac{1}{4}$ we sample $u$ but not $v$, and $v_n$ will not be sampled \vik{Sample $v$ and not $u$ no?}. As such, the total parity of the \mlab edges is odd. Finally, if the number of \mlab edges sampled by $S' \setminus \{u,v\}$ is even and $(u,v)$ have the same parity of \mlab edges connecting to $S' \setminus \{u,v\}$, then with probability at least $\frac{1}{4}$ both $u$ and $v$ are sampled and $v_n$ is sampled. As such, the total parity of the \mlab edges is odd as $(u,v)\in E^-$ and $\Em(v_n, S')$ is even. \vik{Very similar argument to the above. Why is one half of the above not explained to high precision (for being similar) and this one not?}
\item If there is an odd number of vertices sampled from $N^{-}_{G}(v_n)$ in $S'\setminus \{u,v\}$. In this case, if the number of \mlab edges sampled by $S' \setminus \{u,v\}$ is even, then with probability $\frac{1}{4}$, we do not sample neither of $\{u,v\}$ and we sample $v_n$. As such, the total number of \mlab edges is odd. Otherwise, if the number of \mlab edges sampled by $S' \setminus \{u,v\}$ is odd, and $(u,v)$ have different parities of \mlab edges connecting to $S' \setminus \{u,v\}$ (suppose w.log. $v$ has an odd number of \mlab edges); then, with probability at least $\frac{1}{4}$ we sample $u$ but not $v$, and $v_n$ will not be sampled. As such, the total parity of the \mlab edges is odd. Finally, if the number of \mlab edges sampled by $S' \setminus \{u,v\}$ is odd and $(u,v)$ have the same parity of \mlab edges connecting to $S' \setminus \{u,v\}$, then with probability at least $\frac{1}{4}$ both $u$ and $v$ are sampled and $v_n$ is sampled. As such, the total parity of the \mlab edges is odd as $\Em(\{u,v\}, S'\setminus \{u,v\})$ is even, $(u,v)$ plus the \mlab edges in $S'$ is even, and $\Em(v_n, S')$ is odd.
\end{enumerate}
\end{enumerate}

\subsubsection*{The cases in \underline{scenario $(B).$}}
\vik{A reminder for what scenario $(B)$ is would be good here.}
Once again, let us fix all the coins in $S'$ used by line~\ref{line:S-sample-indep} of the $S$-sampler \emph{except} for the special $u$ and $v$ in scenario $(B)$; similar to the analysis in scenario $(A)$, we now sample $u$ and $v$ independently with probability $\frac{1}{2}$ each. We again conduct analysis for different cases.

\begin{enumerate}[label=\Alph*).,leftmargin=1.5cm]
\item The cases when the number of vertices in $S'\setminus \{u,v\}$ is odd:
In such a case, if the number of edges from $\Em$ in $S'\setminus \{u,v\}$ is odd, then with probability $\frac{1}{4}$, we do not sample $u$ or $v$, and $v_{n}$ does not join $S$. As such, we only handle the case when the number of \mlab edges in $S'\setminus \{u,v\}$ is even.
\begin{enumerate}
\item If there is an even number of vertices sampled from $N^{-}_{G}(v_n)$ in $S'\setminus \{v\}$. If the number of \mlab edges between $u$ and $S' \setminus \{u,v\}$ is odd, then with probability at least $\frac{1}{4}$, we sample $u$ but not $v$, and $v_{n}$ will be introduced but the parity will not be flipped. Conversely, if the number of \mlab edges between $u$ and $S' \setminus \{u,v\}$ is even, we look at the parity of the number of \mlab edges between $v$ and $S' \setminus \{u,v\}$. If the number of edges between \mlab edges between $v$ and $S' \setminus \{u,v\}$ is odd, then with probability $\frac{1}{4}$ we sample both $u$ and $v$, and $v_{n}$ does not join $S$, which gives us an odd number of \mlab edges. Otherwise, if the number of edges between \mlab edges between $v$ and $S' \setminus \{u,v\}$ is even, then with probability $\frac{1}{4}$ we sample $v$ but not $u$, and $v_{n}$ joins $S$. As such, we also get an odd number of \mlab edges.
\item If there is an odd number of vertices sampled from $N^{-}_{G}(v_n)$ in $S'\setminus \{u,v\}$. The analysis follows the same logic as in case $(a)$, albeit the parity conditions are flipped.  We omit the excessive repetition of the details.
\end{enumerate}
\item The cases when the number of vertices in $S'\setminus \{u,v\}$ is even:
\begin{enumerate}
\item If there is an even number of vertices sampled from $N^{-}_{G}(v_n)$ in $S'\setminus \{u,v\}$. If the number of \mlab edges sampled by $S'\setminus \{u,v\}$ is odd, then with probability $\frac{1}{4}$, we do not sample $u$ or $v$, and the number of \mlab edges is odd. As such, we only look at the case when the number of \mlab edges sampled by $S'\setminus \{u,v\}$ is even. In such a case, if the \mlab edges between $u$ and $S' \setminus \{u,v\}$ is odd, then with probability at least $\frac{1}{4}$, we sample $u$ but not $v$, and $v_{n}$ will not be introduced. Conversely, if the number of \mlab edges between $u$ and $S' \setminus \{u,v\}$ is even, we look at the parity of the number of \mlab edges between $v$ and $S' \setminus \{u,v\}$. If the number of edges between \mlab edges between $v$ and $S' \setminus \{u,v\}$ is odd, then with probability $\frac{1}{4}$ we sample $v$ but not $u$, and $v_{n}$ does not join $S$, which gives us an odd number of \mlab edges. Otherwise, if the number of edges between \mlab edges between $v$ and $S' \setminus \{u,v\}$ is even, then with probability $\frac{1}{4}$ we sample both $u$ and $v$, and $v_{n}$ joins $S$ to bring an odd number of \mlab edges.
\item If there is an odd number of vertices sampled from $N^{-}_{G}(v_n)$ in $S'\setminus \{v\}$. The analysis follows the same logic as in case $(a)$, albeit the parity conditions are flipped.  We omit the excessive repetition of the details.
\end{enumerate}
\end{enumerate}

Putting all the above cases gives us the desired statement when $G$ is not balanced.
\vik{Done. My vote is to not include this. Even if the mistakes are fixed, I don't see what it adds to anyone's understanding. We also seem to go through flip-graphs next in the app, so why this?}
